# Supplementary material for: RescueAR: Augmented Reality Supported Collaboration for UAV Driven Emergency Response Systems
Source: arXiv:2110.00180 source file (2021-10-01)
Supplement: Supplementary file 1 [file appendix.tex]

\section{Appendix}
\label{sec:appendix}
Step 1: Calculate the E N U values of the point where user touches the screen. \\
E = $World_z - Center_z$ \\
N = $World_x - Center_x$\\
U = 0 \\

Step 2: Calculate the ECEF position of the point where the user touches the screen - The equation is shown below
ENU to ECEF conversion 

% You will have to calculate your ENU origin's ECEF coordinates as well. 

\begin{equation}
\left[\begin{array}{c}
X \\
Y \\
Z
\end{array}\right]=\left[\begin{array}{ccc}
-\sin \lambda & -\sin \phi \cos \lambda & \cos \phi \cos \lambda \\
\cos \lambda & -\sin \phi \sin \lambda & \cos \phi \sin \lambda \\
0 & \cos \phi & \sin \phi
\end{array}\right]\left[\begin{array}{l}
x \\
y \\
z
\end{array}\right]+\left[\begin{array}{c}
X_{r} \\
Y_{r} \\
Z_{r}
\end{array}\right]
\end{equation}
Here the $\phi$ and $\lambda$ values are the geographic latitude and longitude of the drone location, the x,y,z, the  ENU coordinates of where used touched the screen and $X_r$, $Y_r$, $Z_r$ is the ECEF coordinates of the drone location which is calculated as below.
\begin{equation}
\bar{p}=\left[\begin{array}{l}
\bar{p}_{x} \\
\bar{p}_{y} \\
\bar{p}_{z}
\end{array}\right]=\left[\begin{array}{c}
r_{s} \cos \lambda_{s} \cos t+h \cos \mu \cos t \\
r_{s} \cos \lambda_{s} \sin t+h \cos \mu \sin t \\
r_{s} \sin \lambda_{s}+h \sin \mu
\end{array}\right]
\end{equation}

\begin{equation}
    \lambda_{s}=\operatorname{atan}\left((1-f)^{2} \tan \mu\right)
\end{equation}

\begin{equation}
r_{s}=\sqrt{\frac{R^{2}}{1+\left(1 /(1-f)^{2}-1\right) \sin ^{2} \lambda_{s}}}    
\end{equation}
Step 3: Convert the ECEF location calculated in step 2 in to the geo cordinates according to the method described by Zhu\cite{zhu1994conversion} which is best known conversion \footnote{https://en.wikipedia.org/wiki/Geographic\_coordinate\_conversion\#cite\_note-12}
\begin{align}
        r &= \sqrt{X^2 + Y^2} \\[3pt]
     e'^2 &= \frac{a^2 - b^2}{b^2} \\[3pt]
        F &= 54b^2 Z^2 \\[3pt]
        G &= r^2 + \left(1 - e^2\right)Z^2 - e^2\left(a^2 - b^2\right) \\[3pt]
        c &= \frac{e^4 Fr^2}{G^3} \\[3pt]
        s &= \sqrt[3]{1 + c + \sqrt{c^2 + 2c}} \\[3pt]
        P &= \frac{F}{3\left(s + 1 + \frac{1}{s}\right)^2 G^2} \\[3pt]
        Q &= \sqrt{1 + 2e^4 P} \\[3pt]
      r_0 &= \frac{-Pe^2 r}{1 + Q} + \sqrt{\frac{1}{2} a^2\left(1 + \frac{1}{Q}\right) - \frac{P\left(1 - e^2\right)Z^2}{Q(1 + Q)} - \frac{1}{2}Pr^2} \\[3pt]
        U &= \sqrt{\left(r - e^2 r_0\right)^2 + Z^2} \\[3pt]
        V &= \sqrt{\left(r - e^2 r_0\right)^2 + \left(1 - e^2\right)Z^2} \\[3pt]
      z_0 &= \frac{b^2 Z}{aV} \\[3pt]
        h &= U\left(1 - \frac{b^2}{aV}\right) \\[3pt]
     \phi &= \arctan\left[\frac{Z + e'^2 z_0}{r}\right] \\[3pt]
  \lambda &= \operatorname{arctan2}[Y,\, X]
\end{align}
